# Supplementary material for: Achieving Phase-based Logic Bit Storage in Mechanical Metronomes
Source: arXiv:1710.01056 source file (2017-10-03)
Supplement: Supplementary file 1 [file appendixA.tex]

\section{\normalfont Model Code for a Single Metronome}
\applabel{metronome}

 \subsection{\normalfont \texttt{metronomeDAE.m}: model file for metronome DAE in MAPP}
 \applabel{metronome_DAE_code}
 \matlabscript{code/single_metronome_w_input2.m}{lst:metronome_DAE}{\texttt{metronomeDAE.m}}

 \subsection{\normalfont \texttt{metronome.va}: Verilog-A model for a single
 metronome with acceleration input.}
 \applabel{metronome_va_code}
 \verilogascript{code/single_metronome_w_input2.va}{lst:metronome_va}{\texttt{metronome.va}}

\ignore{
 \subsection{\normalfont \texttt{test\_hys.m}: circuit and test script for hys in MAPP}
 \matlabscript{code/test_hys.m}{lst:test_hys_m}{\texttt{test\_hys.m}}

 \subsection{\normalfont \texttt{test\_hys.cir}: circuit and test script for hys in Xyce}
 \verilogascript{code/test_hys.cir}{lst:test_hys_cir}{\texttt{test\_hys.cir}}

 \subsection{\normalfont \texttt{test\_hys.scs}: circuit and test script for hys in \Spectre}
 \verilogascript{code/test_hys.scs}{lst:test_hys_scs}{\texttt{test\_hys.scs}}

 \subsection{\normalfont \texttt{test\_hys.sp}: circuit and test script for hys in \HSPICE}
 \verilogascript{code/test_hys.sp}{lst:test_hys_sp}{\texttt{test\_hys.sp}}

\section{\normalfont Model and Circuit Code for RRAM version 0}
 \subsection{\normalfont \texttt{RRAM\_v0\_ModSpec.m}: model file for RRAM version 0 in MAPP}
 \applabel{RRAM_v0_ModSpec_code}
 \matlabscript{code/RRAM_v0_ModSpec.m}{lst:RRAM_v0_ModSpec}{\texttt{RRAM\_v0\_ModSpec.m}}

 \subsection{\normalfont \texttt{RRAM\_v0.va}: Verilog-A model for RRAM version 0}
 \applabel{RRAM_v0_va_code}
 \verilogascript{code/RRAM_v0.va}{lst:RRAM_v0_va}{\texttt{RRAM\_v0.va}}

 \subsection{\normalfont \texttt{test\_RRAM\_v0.m}: circuit and test script for RRAM version 0 in MAPP}
 \matlabscript{code/test_RRAM_v0.m}{lst:test_RRAM_v0_m}{\texttt{test\_RRAM\_v0.m}}

 \subsection{\normalfont \texttt{test\_RRAM\_v0.cir}: circuit and test script for RRAM version 0 in Xyce}
 \verilogascript{code/test_RRAM_v0.cir}{lst:test_RRAM_v0_cir}{\texttt{test\_RRAM\_v0.cir}}

 \subsection{\normalfont \texttt{test\_RRAM\_v0.scs}: circuit and test script for RRAM version 0 in \Spectre}
 \verilogascript{code/test_RRAM_v0.scs}{lst:test_RRAM_v0_scs}{\texttt{test\_RRAM\_v0.scs}}

 \subsection{\normalfont \texttt{test\_RRAM\_v0.sp}: circuit and test script for RRAM version 0 in \HSPICE}
 \verilogascript{code/test_RRAM_v0.sp}{lst:test_RRAM_v0_sp}{\texttt{test\_RRAM\_v0.sp}}

\section{\normalfont Model Code for Memristor}
 \subsection{\normalfont \texttt{Memristor.m}: model file for memristor ModSpec model in MAPP}
 \applabel{memristor_ModSpec_code}
 \matlabscript{code/Memristor.m}{lst:Memristor}{\texttt{Memristor.m}}

 \subsection{\normalfont \texttt{Memristor.va}: Verilog-A model for Memristor}
 \applabel{memristor_va_code}
 \verilogascript{code/Memristor.va}{lst:Memristor_va}{\texttt{Memristor.va}}

 \subsection{\normalfont \texttt{smoothfunctions.va}: Verilog-A file for smoothing function definitions}
 \applabel{smoothfunctions_va_code}
 \verilogascript{code/smoothfunctions.va}{lst:smoothfunctions}{\texttt{smoothfunctions.va}}
}
